# Supplementary material for: Cross-Lingual Syntactic Transfer with Limited Resources
Source: arXiv:1610.06227 source file (2017-02-04)
Supplement: Supplementary file 1 [file appendix_datasets.tex]

\section{Languages in the Universal Dependencies Experiments}\label{apen_data_sec}
We used the following languages in the universal depdencies corpus: bg (Bulgarian), cs (Czech), da (Danish), de (German), el (Greek), en (English), es (Spanish), et (Estonian), fa (Persian (Farsi)), fi (Finnish), fr (French), hi (Hindi), hr (Croatian), hu (Hungarian), id (Indonesian), it (Italian), la (Latin), nl (Dutch), no (Norwegian), pl (Polish), pt (Portuguese), ro (Romanian), ru (Russian), sl (Slovenian), sv (Swedish), and tr (Turkish).
